# Supplementary material for: MPGM: Scalable and Accurate Multiple Network Alignment
Source: arXiv:1804.10029 source file (2019-05-13)
Supplement: Supplementary file 1 [file suppl_compare.tex]

% !TeX root = suppl.tex

\section{Experimental Evaluations}
